# Supplementary material for: Local and Dimension Adaptive Sparse Grid Interpolation and Quadrature
Source: arXiv:1110.0010 source file (2011-09-30)
Supplement: Supplementary file 1 [file appendix.tex]

\appendix

\section{}
\label{sec:appendix}

\begin{algorithm}
\caption{Generalised Sparse Grid Approximation}
\label{alg:generalisedSG}
\begin{algorithmic}
\STATE $\bi=(0,\ldots,0)$
\STATE $\cA:=\{\bi\}$
\STATE $\cO:=\emptyset$
\STATE $r:=r_\bi$
\WHILE {$r>\varepsilon$}
	\STATE select $\bi \in \cA$ with largest error indicator $r_{\bi}$
	\STATE $\cA:=\cA \setminus \{\bi\}$
	\STATE $\cO:=\cI\cup\{\bi\}$
	\STATE $r:=r-r_\bi$
	\FOR{$k:=1,\ldots,d$}
		\STATE $\bj=\bi+\mathbf{e}_k$
		\IF {$\bj-\mathbf{e}_n \in O \quad \forall\; n=1,\ldots,d$}
			\STATE $\cA:=\cA\cup\{\bj\}$
			\STATE CreateGrid($\bj$)
			\STATE $r:=r+r_\bj$
		\ENDIF
	\ENDFOR
\ENDWHILE
\end{algorithmic}
\end{algorithm}

\begin{algorithm}
\caption{CreateGrid($\bi$)}
\begin{algorithmic}
\label{alg:createGrid}
\FOR{($n\in\{1,\ldots,d\}$)}
  \FOR {($\bx_{\bi-\be_n,\bj} \in \cA_{\bi-\be_n}$ )}
	\STATE $\mathcal{C}$=FindAxialChildren($\bx_{\bi-\be_n,\bj}$,$n$)
	\FOR {( $\bx_{\bi,\bk}\in\mathcal{C}$ )}		
		\IF {( $ \gamma_{\bi,\bk} \ge \varepsilon$ )}
			\STATE $\cA_{\bi}:=\cA_\bi\cup\{\bx_{\bi,\bk}\}$
		\ELSE 
			\STATE $\cR_\bi:=\cR_\bi\cup\{\bx_{\bi,\bk}\}$
		\ENDIF
	\ENDFOR
  \ENDFOR
\ENDFOR
\end{algorithmic}
\end{algorithm}
